# Supplementary material for: Single-bubble and multi-bubble cavitation in water triggered by laser-driven focusing shock waves
Source: arXiv:1709.06836 source file (2018-03-29)
Supplement: Supplementary file 1 [file Supplemental.pdf]

# Supplemental Material for “Single-bubble and multi-bubble cavitation in water triggered by laser-driven focusing shock waves”

D. Veysset,<sup>1,2</sup> U. Gutiérrez-Hernández,<sup>3</sup> L. Dresselhaus-Cooper,<sup>1,2</sup> F. De  
Colle,<sup>3</sup> S. Kooi,<sup>2</sup> K. A. Nelson,<sup>1,2</sup> P. A. Quinto-Su,<sup>3,\*</sup> and T. Pezeril<sup>4,†</sup>

<sup>1</sup>*Department of Chemistry, Massachusetts Institute of Technology, Cambridge, MA 02139, USA*

<sup>2</sup>*Institute for Soldier Nanotechnologies, Massachusetts Institute of Technology, Cambridge, MA 02139, USA*

<sup>3</sup>*Instituto de Ciencias Nucleares, Universidad Nacional Autónoma de México,  
Apartado Postal 70-543, 04510 Cd. Mx., México*

<sup>4</sup>*Institut Molécules et Matériaux du Mans, UMR CNRS 6283, Université du Maine, 72085 Le Mans, France*

## I. SINGLE SHOT MULTI-FRAME IMAGING, TERTIARY BUBBLE CLOUD

The characteristic timescale of collapse for a selection of bubbles from the tertiary bubble cloud is displayed in Fig. S1. The fast collapse of the tertiary bubbles of very small diameters, in the order of 10 microns or smaller, suggests that those bubbles remain in the bulk of the water and are spherical.

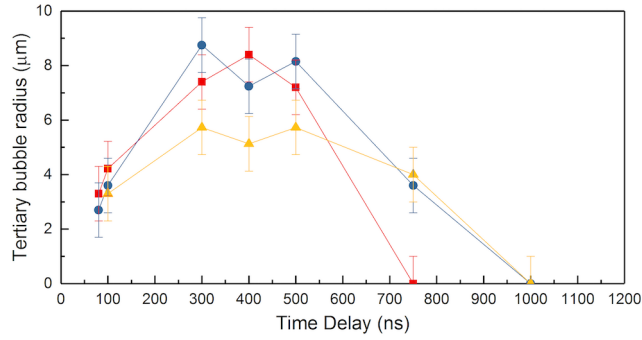

Fig. S1 : Bubble radii as a function of time for a selection of three most visible bubbles (blue, red, and yellow) from the tertiary bubble cloud, extracted from Fig. 2.

## II. SINGLE SHOT STROBOSCOPIC IMAGING, EXPERIMENTS VARYING THE LASER RING RADIUS

Figure S2 shows the dynamics of the annular laser-induced bubbles and the shock-induced central bubbles as a function of laser radius. Each row corresponds to a different value for the laser ring radius  $R$  (55, 68, 80, 92, and 105  $\mu\text{m}$ ), with the smallest being at the top row, while the columns corresponds to different time delays. The central column in Fig. S2 shows images of the inner shock that focuses at the center of the laser ring. As expected, the time for shock focusing increases when the laser ring radius  $R$  increases. At longer time delays, the diverging inner shock and a cavitation bubble growing at the center can be seen on the right column of images displayed in Fig. S2. Once the inner diverging shock reaches the wall of the annular laser-induced bubble, it is reflected as a tensile shock wave and travels back toward the center of the ring.

As evidenced in Fig. S3, a tertiary bubble cloud such as the one observed in Fig. 2, appears on a time scale following the reflection of the diverging inner shock at the annular laser-induced bubble wall. These observations suggest that the rebounding shock wave becomes negative upon reflection at the annular laser-induced bubble wall due to the

---

\*Electronic address: [pedro.quinto@nucleares.unam.mx](mailto:pedro.quinto@nucleares.unam.mx)

†Electronic address: [thomas.pezeril@univ-lemans.fr](mailto:thomas.pezeril@univ-lemans.fr)

acoustic impedance mismatch between the liquid and the bubble, which leads to the nucleation of a tertiary bubble cloud. We also observe that the nucleated bubble clouds are larger for smaller laser excitation rings, see the frames bounded by dashed lines in Fig. S3. For instance, for the laser ring radius  $R$  of  $55\text{ }\mu\text{m}$  and  $68\text{ }\mu\text{m}$ , the bubble clouds fully fill the space enclosed by the annular laser-induced bubble, see at  $132\text{ ns}$  time delay in Fig. S3. We also speculate that the annular laser-induced bubble increases the lifetime of the nucleated bubble clouds [1] by shielding the microbubbles from the liquid static pressure. It seems as well that multiple bubble clouds are nucleated as the reflected inner tensile shock focuses towards the center. Most probably, the bubble clouds in Fig. S3 have a sufficiently long lifetime for several bubble clouds to appear simultaneously while the shock bounces back and forth inside the annular laser-induced bubble.

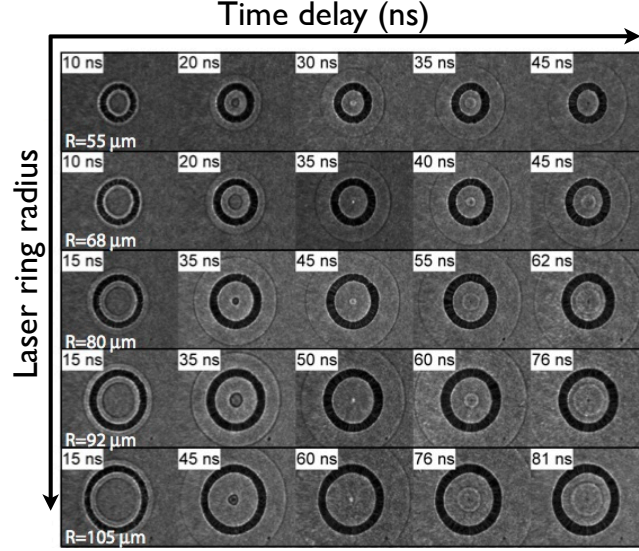

Fig. S2 : Single-shot stroboscopic time-resolved images recorded for different laser ring radii  $R = 55, 68, 80, 92, 105\text{ }\mu\text{m}$ . Each individual frame has a width of  $410\text{ }\mu\text{m}$ . The central column shows the instant of inner shock focus.

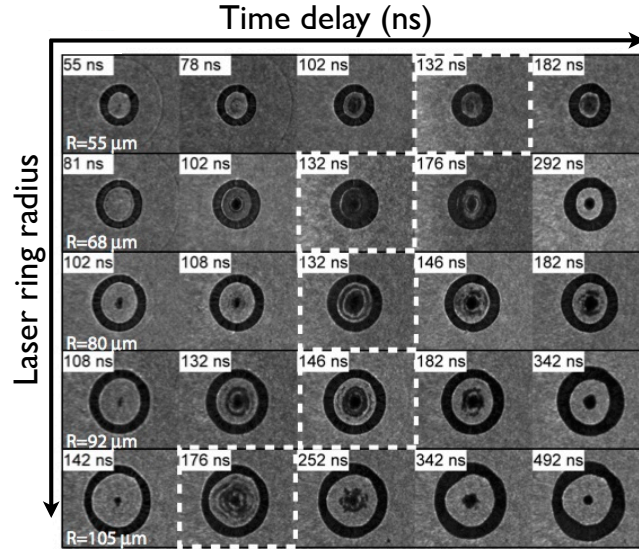

Fig. S3 : Stroboscopic time-resolved images recorded such as in Fig. S2, at longer timescales. A bubble cloud appear after reflection of the inner shock at the annular laser-induced bubble. The dashed frames highlight the instant when the bubble cloud appears to be largest. Each individual frame has a width of  $410\text{ }\mu\text{m}$ .

### III. FAR FIELD SIMULATIONS

The analytical solution for a ring piston in cylindrical coordinates, as written in Blackstock [2] decays as  $1/r$  in the far field. Accordingly, we have run additional numerical simulations at much longer distances from the ring, to explore the far-field limit and compare our numerical results with the analytical theory. The results of a low amplitude shock with an initial pressure of 1MPa are presented in Fig. S4. The numerical simulations agree perfectly with the analytical theory. We observe that the maximum pressure decays as  $1/r$  as soon as the shock propagation distance reaches about 300 microns and beyond. The agreement between the analytical theory and the simulations confirm the accuracy of our numerical modeling, that can simulate low to strong shock waves, at short distances or long distances.

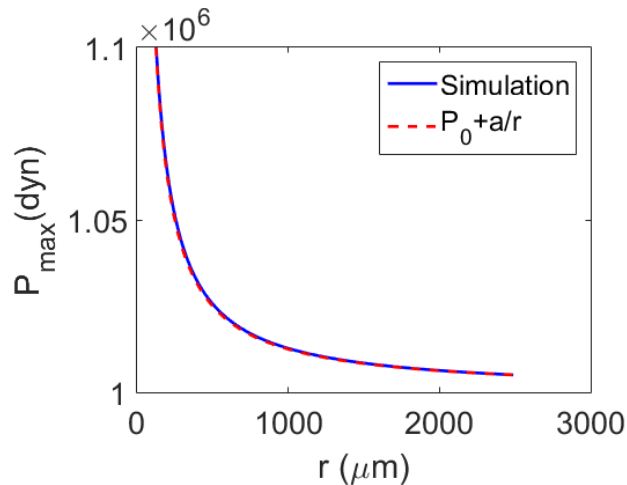

Fig. S4 : Plot of the maximum pressure evolution at long distances and analytical fit following  $a/r$  with  $a = 1250$  Pa.

- 
- [1] N. Bremond, M. Arora, C.D. Ohl, D. Lohse, Phys. Rev. Lett. **96**, 224501 (2006).
  - [2] D. T. Blackstock, *Fundamentals of Physical Acoustics*, John Wiley & Sons (2000).
